# Supplementary material for: DISTA-Net: Dynamic Closely-Spaced Infrared Small Target Unmixing
Source: arXiv:2505.19148 source file (2025-12-10)
Supplement: Supplementary file 1 [file 10-Supplementary.tex]

\clearpage
\begin{center}
\textbf{{\Large Supplementary}}
\end{center}
\setcounter{section}{0}

\section{Optical Imaging Models}\label{appendix:Imaging}

\begin{figure*}[htbp]
    \centering
    \includegraphics[width=0.85\textwidth]{../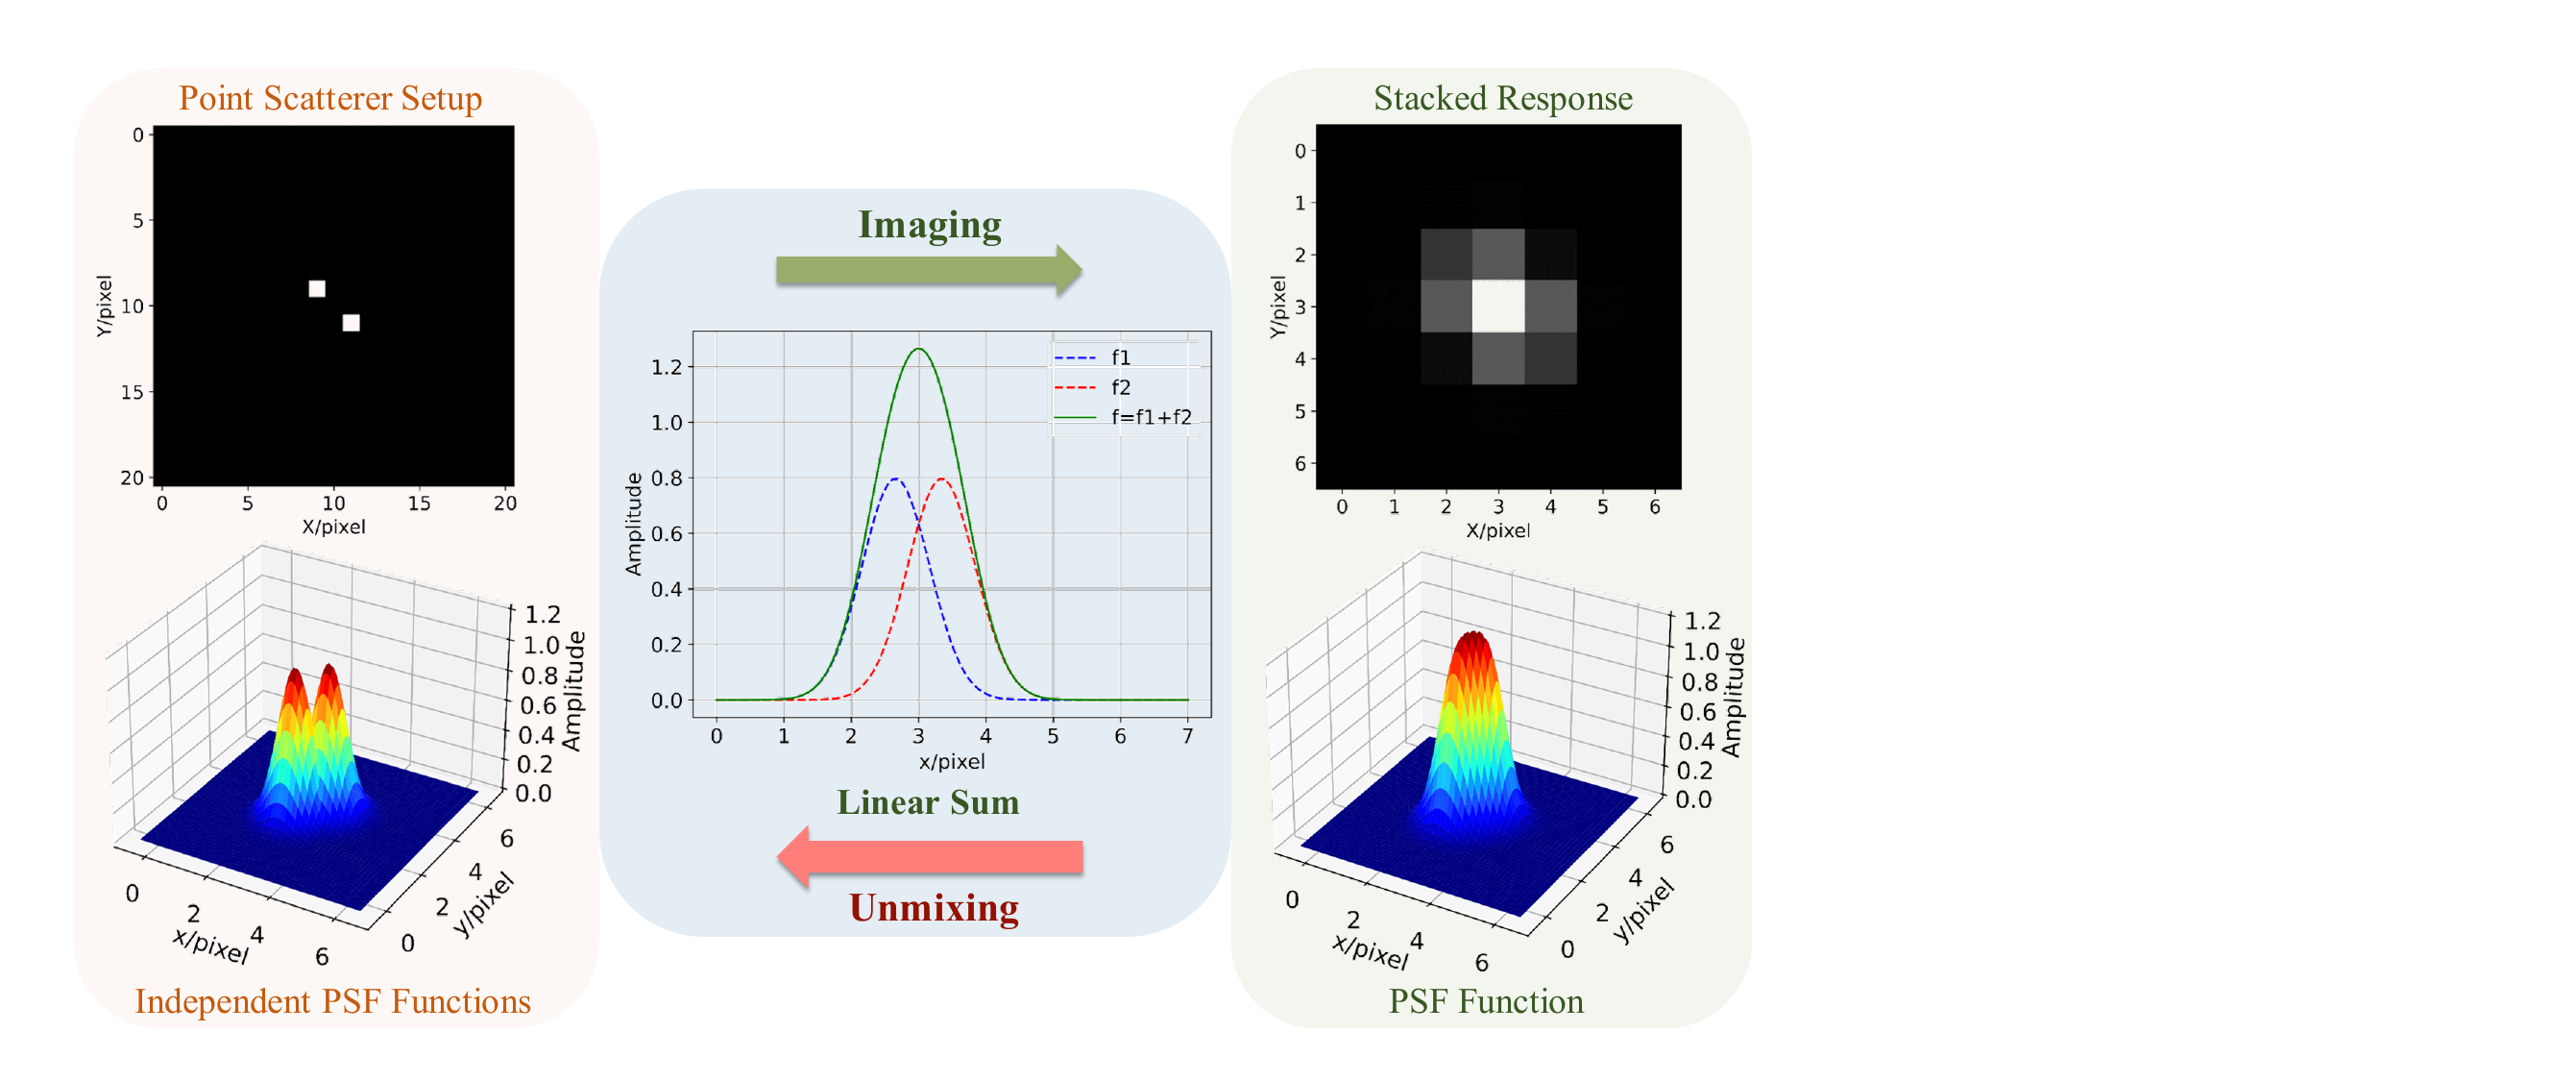}
    \caption{Multi target imaging, the imaging of distant targets on the image plane can be regarded as the diffusion of energy by point source targets through PSF. Multi target imaging is the cumulative response of superimposed point sources.}
    \label{fig:linear_sup}
\end{figure*}
When a point light source is imaged through a lens, a diffraction pattern called the "Airy disk" forms at the focal point, featuring a bright central spot surrounded by concentric rings of alternating bright and dark fringes.
This effect is approximated by the point spread function (PSF), whose standard deviation, dependent on the sensor's focal ratio ($f$-number) and detection band, quantifies the energy spread. In multi-target imaging,  each pixel's intensity is the cumulative response of overlaid point sources. The detector receives a combined energy response that is the linear sum of individual PSFs . This superposition principle is fundamental to the CSIST unmixing process, where the stacked response must be decomposed to identify and characterize closely-spaced infrared targets, as illustrated in Fig.~\ref{fig:linear_sup}.
For remote objects, each acts as a point source, with the radius of the resultant Airy spot dictated by $1.22 \lambda/D$, where $\lambda$ is the wavelength and $D$ the lens diameter.
This radius is equivalent to $1.9\sigma$ of a Gaussian PSF, defining the sensor's physical resolution limit per the Rayleigh criterion.

 % When targets are at considerable distances, they can be approximated as point sources, with their energy distribution on the sensor's focal plane characterized by Point Spread Functions (PSFs) that approximate two-dimensional Gaussian functions. 

\section{CSO-mAP Metric}\label{appendix:metric}
Once the predictions are classified as TP or FP, a binary list is constructed following the common practice in COCO, where a TP prediction is indicated by 1 and an FP prediction by 0. 
This binary list serves as the foundation for generating the Precision-Recall (PR) curve.
By varying the intensity threshold for positive predictions, a series of Precision and Recall values are obtained, forming the PR curve. 
The Average Precision (AP), calculated as the area under the PR curve, provides a comprehensive assessment of the model's performance across various intensity thresholds, effectively summarizing the trade-off between Precision and Recall.
Finally, we introduce the CSO mean Average Precision (CSO-mAP), which averages the AP across different distance thresholds $\delta_k$, offering a standardized metric for comparing the performance of models in the CSIST unmixing task.

\section{GrokCSO Toolkit}\label{appendix:toolkit}
Recognizing the void in specialized, accessible tools for this domain, we introduce GrokCSO, a comprehensive, open-source toolkit architected to enhance the reconstruction of closely spaced infrared small targets. While generic computer vision fields benefit from a plethora of object detection toolkits like MMDetection and GluonCV, the specificity of infrared small target unmixing has long necessitated a dedicated platform. The absence of such a platform has fragmented research efforts, impeding the reproducibility of experiments and the comparative analysis of algorithms.

Developed atop the robust PyTorch framework, GrokCSO is meticulously designed to address the unique challenges inherent to closely spaced infrared small target unmixing. It stands distinguished in its offerings:
\begin{compactenum}
  \item \textbf{Pre-trained Models and Reproducibility}: GrokCSO equips researchers with an arsenal of pre-trained models, complete with training scripts and logs of leading-edge algorithms. This repository of resources not only fosters reproducibility but also facilitates nuanced comparisons across diverse algorithmic approaches.
  \item \textbf{Tailored Flexibility and Evaluative Rigor}: With an extensive suite of adaptable backbones and necks, GrokCSO accommodates a broader spectrum of computational strategies. The toolkit incorporates specialized dataset loaders, cutting-edge attention mechanisms, and versatile data augmentation workflows. Moreover, GrokCSO introduces evaluation metrics specifically calibrated for the intricacies of closely spaced infrared small target unmixing. These metrics honor the distinct nature of CSO challenges.
\end{compactenum}

\section{Hyperparameters Analysis}\label{ana}

\begin{figure}[htbp]
\centering
\includegraphics[width=.45\textwidth]{../figs/experiment/Line chart1.pdf}
\caption{CSO-mAP performance under different Stage Numbers and Branch coefficients.}
\label{fig:linechart1}
\end{figure}

We also conduct experiments to analyze the relationship between model performance, the number of stages, and the coefficient of the dynamic transform branch, validating its architectural and parametric robustness.

First, to determine an appropriate number of stages, we trained the network with stage numbers \( K = 2, 4, 6, 8, \) and \( 10 \). The performance curves are recorded in Figure~\ref{fig:linechart1}. As the number of stages increases from 2 to 6, the CSO-mAP score improves, reaching its peak (46.74\%) at 6 stages. Beyond this point, additional stages result in diminishing returns. Therefore, selecting 6 stages provides an optimal balance between accuracy and efficiency.

Second, we adjusted the proportion of the dynamic transform branch relative to the total contribution of both branches and observed the performance changes. Starting from 0\% coefficient, performance improves as the influence of the dynamic branch increases, peaking at a 30\% coefficient. The model maintains stable performance across coefficient settings from 50\% to 90\%, demonstrating robustness. However, at 100\% coefficient, performance drops sharply to 30.62 (not labeled in the figure), confirming that integrating both branches is crucial for optimal feature representation.

\section{Initialization and Learning Objectives.}\label{appendix:loc}

\noindent \textbf{Initialization.} \label{appendix:init}
Given a dataset $\{(z_i, s_i)\}_{i=1}^M$, where $z_i$ is an image of overlapping targets and $s_i$ is the corresponding super-resolved image, we calculate high-resolution target coordinates in $s_i$ using the target information $(x_i, y_i, g_i)$ and a scaling factor $c$. For instance, the grayscale value $g_i$ at position $(c \cdot x_i + \frac{c-1}{2}, c \cdot y_i + \frac{c-1}{2})$ in the high-resolution image is used to generate $s_i$.

Let \(Z = [z_1, \ldots, z_M]\) and \(S = [s_1, \ldots, s_M]\). The matrix \(Q_{\text{init}}\) for initializing \( \tilde{s}^{(0)} \) is computed as:
\begin{equation*}
    Q_{\text{init}} = \arg \min_Q \|QZ - S\|_F^2 = SZ^T (ZZ^T)^{-1}.
\end{equation*}
Thus, \( \tilde{s}^{(0)} \) is given by:
\begin{equation*}
    \tilde{s}^{(0)} = Q_{\text{init}} Z.
\end{equation*}

\noindent \textbf{Loss Function.} \label{appendix:loss}
To ensure that the unmixed image \( \tilde{s} \) is as close as possible to the ground truth image \( s \) while maintaining the structure \( \tilde{\mathcal{F}}(\cdot) \circ \mathcal{F}(\cdot) = \mathbf{I} \), we designed the following end-to-end training loss function for DISTA-Net, with a training dataset of size \( M \), \( N \) stages, and image size \( N_s \):
\begin{equation*}
    \mathcal{L} = \mathcal{L}_{\text{discrepancy}} + \gamma \mathcal{L}_{\text{constraint}},
\end{equation*}
where:
\begin{equation*}
    \mathcal{L}_{\text{discrepancy}} = \frac{1}{M N_s} \sum_{i=1}^M \| \tilde{s}_i^{(N)} - s_i \|_2^2,
\end{equation*}
\begin{equation*}
    \mathcal{L}_{\text{constraint}} = \frac{1}{M N_s} \sum_{i=1}^M \sum_{k=1}^N \| \tilde{\mathcal{F}}^{(k)} (\mathcal{F}_d^{(k)} (s_i)) - s_i \|_2^2.
\end{equation*}
Here, \( L_{\text{discrepancy}} \) measures the mean squared error (MSE) between the super-resolved image \( \tilde{s}_i^{(N)} \) and the ground truth image \( s_i \). \( L_{\text{constraint}} \) enforces the structural constraint by ensuring that the composition of \( \tilde{\mathcal{F}}^{(k)} \) and \( \mathcal{F}^{(k)} \) approximates the identity transformation for each stage \( k \). \( \gamma \) is a parameter that balances the discrepancy and constraint terms.

This loss function aims to balance the accuracy of the unmixed images with the structural integrity of the transformation functions.
